# Supplementary material for: Bermuda: Bidirectional de novo assembly of transcripts with new insights for handling uneven coverage
Source: arXiv:1506.05538 source file (2015-06-18)
Supplement: Supplementary file 1 [file Supplementary_Method.pdf]

Supplementary Information for the following manuscript:

Qingming Tang, Sheng Wang, Jian Peng, Jianzhu Ma and Jinbo Xu. Bermuda: Bidirectional de novo assembly of transcripts with new insights for handling uneven coverage

## 1. Data structures for De Bruijn graph in memory

We use a  $(k+1)$ -mer to represent an edge in a  $k$ -mer de Bruijn graph. Due to sequencing errors, there may be a huge number of different  $(k+1)$ -mers when  $k$  is big (e.g.,  $k=30$ ). To achieve a tradeoff between memory consumption and running time, we store the edges (i.e., the  $(k+1)$ -mers) in both hash tables and balanced trees. A hash table offers almost a constant retrieval time, but may contain many unused entries and thus, waste some memory. This may prevent our software from running on a computer with relatively small physical memory. A balanced tree does not contain any unused nodes, but offers only a logarithmic retrieval time. In summary, we use hash tables to store most of the  $(k+1)$ -mers appearing only once in the reads while balanced trees for the remaining  $(k+1)$ -mers.

Let  $\text{Pre}(X)$  and  $\text{Suf}(X)$  denote the prefix and suffix of a  $(k+1)$ -mer  $X$ , respectively. By default,  $\text{Pre}(X)$  contains the first 5 bps of the  $(k+1)$ -mer and  $\text{Suf}(X)$  the remaining bps. Accordingly, we use  $4^5$  hash tables and balanced trees to store a  $k$ -mer de Bruijn graph.  $X$  is stored in either a hash table or a balanced tree indexed by  $\text{Pre}(X)$ . Each node in a balanced tree corresponds to one  $(k+1)$ -mer, consisting of two components:  $\text{Suf}(X)$  and the occurring frequency of  $X$  in the reads. Let  $H(X)$  denote the hash value of  $\text{Suf}(X)$ . For any  $(k+1)$ -mer  $X$ , if it appears more than once or there is another  $(k+1)$ -mer  $X'$  such that  $H(X)=H(X')$ , we add  $X$  to a balanced tree, otherwise to a hash table indexed by  $\text{Pre}(X)$ .

## 2. Parallel path detection algorithm

There may be more than two parallel paths between a pair of given nodes since one position could be mistakenly sequenced in several different ways. We design a heuristic parallel path search algorithm which can identify multiple parallel paths among two nodes, and also those complicated parallel paths (e.g. paths share internal nodes with some true paths). Our path search algorithm is based upon the observation that there are far fewer parallel paths (than the total number of paths) and that two parallel paths differ from each other by only a very small number of positions, so we can apply a pruning strategy at early stage to save running time. Let  $\text{ExpandList}$  and  $\text{ParaPaths}$  denote the set of paths that could be potentially expanded into parallel paths and the set of identified parallel paths, respectively. Given a node  $u$  as input, our search algorithm detects all the parallel paths starting from  $u$  as follows.

Step 1: Let  $v_1, v_2, \dots, v_t$  ( $t \leq 4$ ) denote all the nodes pointed to by the node  $u$ . If  $t < 1$ , our algorithm terminates and returns no parallel path at all. Otherwise, we add  $\frac{(t-1)t}{2}$  node pairs  $(v_1, v_2), (v_1, v_3), \dots, (v_1, v_t), \dots, (v_{t-1}, v_t)$  to  $\text{ExpandList}$ . Each node in a pair is a path, which may be expanded into one parallel path later.

Step 2: Remove one path pair  $(P_i, P_j)$  from ExpandList. Let  $X_i$  and  $X_j$  denote the sets of nodes pointed to by the last nodes of the paths  $P_i$  and  $P_j$ , respectively. For any two nodes  $x_i \in X_i$  and  $x_j \in X_j$ , we append  $x_i$  and  $x_j$  to  $P_i$  and  $P_j$ , respectively, to form a pair of new paths  $Q_i$  and  $Q_j$ . There are three cases.

Case 1. If  $x_i$  is the same as  $x_j$ , then  $Q_i$  and  $Q_j$  form a pair of parallel paths. We add the pair  $(Q_i, Q_j)$  to ParaPaths.

Case 2. If  $x_i$  is different from  $x_j$  but  $Q_i$  and  $Q_j$  are still very similar, we add the pair  $(Q_i, Q_j)$  to ExpandList since  $Q_i$  and  $Q_j$  could be expanded to a pair of parallel paths later.

Case 3. If  $Q_i$  and  $Q_j$  are quite different,  $Q_i$  and  $Q_j$  cannot form a pair of parallel paths. Therefore, we just discard this path pair.

Step 3. We repeat Step2 until ExpandList is empty. Afterwards, we cluster all the parallel paths in ParaPaths. In each cluster we treat the path with the largest read support as the correct one and the others as erroneous.

Step 2 runs fast since cases 1 and 3 occur much more frequently than case 2 (because two parallel paths differ only in very few positions). To speed up Step 2, we keep only those path pairs with  $\min(\frac{|Q_j|}{|Q_i|}, \frac{|Q_i|}{|Q_j|})$  smaller than 0.2, where the notion  $| \cdot |$  denotes the number of reads supporting one path. The underlying intuition is that if  $Q_i(Q_j)$  is a variant of  $Q_j(Q_i)$  due to sequencing errors, their support ratio shall not deviate too much from the sequencing error ratio.

### 3. Read correction with 'N's

The main text describes how to correct errors in reads without considering 'N's. When there are 'N's in sequences, we correct read errors as follows:

- 1) We divide a sequence into segments at all the 'N' positions and then correct each segment using the method described in the main text. If the total number of errors in the sequence is no larger than a given threshold (2 by default), the sequence is corrected and kept, otherwise discarded.
- 2) For any two adjacent segments with  $x$  'N's in between, if in the de Bruijn graphs we can find a unique path with length  $x$  connecting these two segments, then we replace the  $x$  'N's by this path to form a corrected read.

### 4. More details for fragment construction

#### Determining if the Source and Target shall be connected or not

When using reverse direction construction, we need to determine if the Source and the Target are connected or not. When there is a number  $L$  ( $5 < L < k_{min}$ ) such that the  $L$ -length prefix of the Target is exactly same as the  $L$ -length suffix of the Source, the Source and the Target shall be connected. To tell if this condition holds or not, we first construct the suffix tree using the last  $k_{min}$  bases of the Source. Then, we find a path in the suffix tree that exactly matches the prefix of the Target, as shown in Figure S4A. If the path length is between 5 and  $k_{min}$ , the Source and Target are connected and merged together. Otherwise, the Source and Target are still disconnected.

### **Fragment growth using nodes in the Target**

After the last node of the Source has been examined, we set one node in the Target as red node and continue the basic fragment construction process. When the Source and Target are not connected (Figure S4B), we set the first node of the Target as the red node and the following nodes as blue. When the Source and Target are already connected (Figure S4C), we set the first node in the Target but not in the Source as the red node and the following nodes as blue.
